# Supplementary material for: Network Friendly Recommendations: Optimizing for Long Viewing Sessions
Source: arXiv:2110.00772 source file (2021-10-02)
Supplement: Supplementary file 1 [file appendixA.tex]

\subsection{Proof of Lemma~\ref{lemma:rec-cost}}

Let a user start a sub-sequence by retrieving content $i$. The expected number of retrievals of content $j$ (or, number of times visiting state $j$) until the end of the sub-sequence is given by $g_{ij}$, where $g_{ij}$ is the ($i$-row,$j$-column) element of the \textit{fundamental matrix} $\mathbf{G}$ of the AMC~\cite{grinstead2012introduction}.
The \say{fundamental matrix} is defined as

\begin{equation}\label{eq:fundamental-matrix-definition}
\mathbf{G} = \textstyle\sum_{n=0}^{\infty} \mathbf{Q}^{n} = (\mathbf{I}-\mathbf{Q})^{-1}
\end{equation}

% where $\mathbf{Q}$ the matrix with the transition probabilities $q_{ij}$ between the transient states of the AMC ($i,j\in\mathcal{K}$). 

where obviously $q_{ij} = \frac{\alpha}{N}\cdot r_{ij}$ as defined from \eq{eq:transition-matrix}.
% \pavlos{be careful - ref}
%\end{equation}
Substituting this into \eq{eq:fundamental-matrix-definition} gives the expression for $\mathbf{G}$ that appears in Lemma~\ref{lemma:rec-cost}.

Now, the cost of retrieving a content $j$ is $c_{j}$. Since each content $j$ is retrieved on average $g_{ij}$ times during a sub-sequence that starts from $i$, the total cost is given by 

\begin{equation}
E[C(S_{R})~|~ i] = \textstyle\sum_{j\in\mathcal{K}} g_{ij}\cdot c_{j}
\end{equation}

The probability that a sub-sequence starts at content $i$ is equal for all sub-sessions and is given by $p_{i}$. Thus, taking the expectation over all the possible initial states $i$, gives

\begin{equation}
E[C(S_{R})] = \sum_{i\in\mathcal{K}} E[C(S_{R})~|~ i] \cdot p_{0}(i) = \sum_{i\in\mathcal{K}} \sum_{j\in\mathcal{K}} g_{ij}\cdot c_{j} \cdot p_{0}(i)
\end{equation}

Expressing the above summation as the product of the vectors $\mathbf{p}_{0}$ and $\mathbf{c}$, and the matrix $\mathbf{G}$, gives \eq{eq:cost-cycle}.
Similarly, if $g_{ij}$ is the amount of time spent on state $j$ before absorption, starting from state $i$, then $\sum_{j} g_{ij}$ must be equal to the total time spent at \emph{any state} before absorption% (starting again from state $i$)
. Weighing this with the probability $p_{0}(i)$ of starting at each state $i$, gives the expected time to absorption, which is the expected duration of a sub-sequence $E[|S_{R}|] = \sum_{i} p_{0}(i) \cdot \sum_{j} g_{ij}$. Writing this in matrix notation, gives the first part of Eq.(\ref{eq:cycle-length}). 
However, observe that the probability of absorption at any state $i$ is equal to $1-\alpha$, independent of $i$. Hence, the number of steps till absorption is a geometric random variable with parameter $1-\alpha$, and thus the mean time to absorption is $\frac{1}{1-\alpha}$.

\subsection{Problem Convexification for the Non-Uniform Case}

% Notice that the Remark \ref{remark:convex} gives us some intuition and explains why the the non-uniform pppmf case of the problem has the same structure with the \probref{problem:basis}.
We perform the same intermediate step as in Section \ref{sec:optimization_methodology}, that is we set
\begin{align}
\mathbf{z}^T = \mathbf{p}_0^T \cdot (\mathbf{I} - \alpha \sum_{n = 1}^N v_n \mathbf{R}^n)^{-1} \Rightarrow \mathbf{z}^T - \alpha \cdot \mathbf{z} \sum_{n=1}^N v_n \mathbf{R}^n = \mathbf{p}_0^T 
\end{align}
according to which we still have a nonconvex problem. That is the spot where we need to use the \say{convex combination} argument, and intuitively set $f_{ij}^{n} = z_i \cdot r_{ij}$ as in the previous section. Regarding the problem constraints, we know that since we incorporated only new \emph{linear} constraints, our transformation will not affect them.
Therefore, \nameref{problem:nuct} can be also transformed into an LP and be written as
\begin{problem}[LP(OP-pref)]\label{problem:ltecnu-lp}
\begin{subequations}
\label{eq:objective-LP}
\begin{align}
\underset{\mathbf{z},~\mathbf{F}^{1},..,\mathbf{F}^{N}}{\textnormal{minimize}} ~~~ & 
  \mathbf{c}^T \cdot \mathbf{z}, \label{new-obj2}\\
\textnormal{subject to} \quad & \sum_{j =1}^{K} \sum_{n=1}^{N} v_{n} \cdot f^{n}_{ij} \cdot u_{ij} \geq z_i \cdot q \cdot q_i^{max},~\forall~i~\in \mathcal{K}
\label{quality-con-LP}\\
& \sum_{j = 1}^{K} f^{n}_{ij} = z_i , ~\forall~i~\in \mathcal{K}~\textnormal{and}~n=1,..,N \label{affine-con-LP}\\
& \sum_{n = 1}^{N} f^{n}_{ij} \le z_i,~\forall~\{i,~j\} \in \mathcal{K} \label{implementable-lp} \\
& f^{n}_{ij} \ge 0 \; (i \neq j), \;\; f^{n}_{ii} = 0, \forall~i,j~\in~\mathcal{K} \label{f-positive-con-LP}\\
&	z_j - \alpha \cdot \sum_{n=1}^{N} v_n \sum_{i}^{K}f^{n}_{ij} = p_{0}(j), ~\forall~j \in \mathcal{K} \label{zf-relaxation}
\end{align}
\end{subequations}
\end{problem}
