# Supplementary material for: Network Friendly Recommendations: Optimizing for Long Viewing Sessions
Source: arXiv:2110.00772 source file (2021-10-02)
Supplement: Supplementary file 2 [file appendixB.tex]

Assume a linear function $f:\mathbb{R}^{K} \rightarrow \mathbb{R}$ of the form
$f(\mathbf{x})=\sum_{i=1}^{K} c_{i} \cdot x_{i}$ with $c_{i} \ge 0~\forall~i$ and $c_1 < ...< c_K$ (sorted in increasing order). 

\begin{align}
f(\mathbf{x}) = c_{1} x_1 +...+ c_{K} x_K = c_1(x_1+...\frac{c_K}{c_1}x_K) \\ \nonumber \Leftrightarrow \frac{1}{c_1}f(\mathbf{x}) = x_1 +\frac{c_{2}}{c_1}x_2...+\frac{c_{K}}{c_1}x_K
\end{align}

We are interested in finding the minimum of this function, whose solution \emph{must also lie} in the set $\mathcal{S}= \{x_i:~\sum_{i=1}^{K} x_{i} = 1~\text{and}~x_i\ge0\}$. Since we need the minimum we can allow $\sum_{i=1}^{K} x_{i} \ge 1$, as the solution \emph{will not} become unbounded. 
\begin{equation}
x_1 +...+  x_K \ge 1 
\end{equation}
We add to both sides of the inequality the quantities $\frac{c_i-c_{1}}{c_1}\cdot x_i~\forall~i$.
This will result the following.

\begin{align}
\frac{1}{c_1}f(\mathbf{x}) \ge 1+ \frac{c_{2}-c_1}{c_1}x_2+...+\frac{c_{K}-c_1}{c_1}x_K 
\end{align}

It is easy to see that since $c_{i}-c_{1},x_{i}\ge0$, the optimal value for $f(\mathbf{x})$ is obtained by assigning $x_{2}=...=x_{K}=0$. Therefore, we need to assign $x_1=1$, which was the variable paired with the lowest coefficient, and at that case the minimum value is exactly $c_1$.
Note that here, we proved the case where the equality constraint is equal to 1; if we had an equality with $N>1$, it is trivial to see that the exact same procedure repeated $N$ time would return the optimal.
